# Supplementary material for: Relation-aware Video Reading Comprehension for Temporal Language Grounding
Source: arXiv:2110.05717 source file (2021-12-01)
Supplement: Supplementary file 1 [file appendix.tex]

\subsubsection{Different operators used in Multi-Choice Generator}
 We conduct experiments to reveal the effect of different generators. For a moment candidate $<t^s_i, t^e_i>$, it has the corresponding feature sequence $Y$ from $\hat{\mathbf{V}}$ denoted as $Y=\{\hat{v}_k\}_{k={t^s_i}}^{t^e_i}$. We explore four types of operators (\ie, pooling, sampling, concatenation and addition, ) in the multi-choice generator. The first two consider all the information of the region within the temporal span of the candidate. Pooling operator focuses on the statistic characteristic and the sampling serves as weight average operator. However, the last two only consider the boundary information ($v_{t^s_i}$ and $v_{t^e_i}$) of a moment candidate, which expect the cross-modal interaction to be boundary sensitive. Table \ref{tab:abs_tacos} reports the performance of different operators on TACoS dataset. It is observed that concatenation operator achieves the highest score across all the evaluation criterion which indicates boundary sensitive operators have better performance than the statistical operators.

\begin{table}[t]
    \centering
    \begin{tabular}{ccccc}
    \toprule
    \multirow{2}{*}{\textbf{Operators}} & \multicolumn{2}{c}{\textbf{Rank1@}}  & \multicolumn{2}{c}{\textbf{Rank5@}} \\
         & \textbf{0.3} & \textbf{0.5} &\textbf{0.3} & \textbf{0.5} \\
    \midrule
    Pooling &  40.61& 29.62 & 64.58 & 52.79 \\
    Sampling&  41.33& 30.82 & 65.53 & 53.54 \\
    Addition &  42.04& 31.22 & 63.86 & 51.24 \\
    Concatenation & \textbf{43.09} & \textbf{32.24} & \textbf{68.71} & \textbf{55.51} \\
    \bottomrule
    \end{tabular}
    \caption{Effectiveness of different operators used in Multi-Choice Generator on TACoS, measured by \textit{Rank 1@$\mu \in\{0.3, 0.5\}$} and \textit{Rank 5@$\mu \in\{0.3, 0.5\}$}.}
    \label{tab:abs_tacos}
\end{table}

\subsubsection{Performance Comparison with State-of-the-arts}
In this section, we show the whole tables of performance comparison with state-of-the-arts methods, which are not fully shown in the body paragraph for saving space.

\begin{table}[t]
    \centering
    \footnotesize
    \begin{tabular}{ccccccc}
    \toprule
    \multirow{2}{*}{\textbf{Methods}} & \multicolumn{3}{c}{\textbf{Rank1@}}  & \multicolumn{3}{c}{\textbf{Rank5@}} \\
    & \textbf{0.1} & \textbf{0.3} & \textbf{0.5} & \textbf{0.1} & \textbf{0.3} & \textbf{0.5} \\
    \midrule
    MCN & 14.42 &  - & 5.58 & 37.35 & - & 10.33\\
    CTRL & 24.32 & 18.32 & 13.30 & 48.73 & 36.69 & 25.42 \\
    TGN & 41.87 & 21.77 & 18.9 & 53.40 & 39.06 & 31.02 \\
    MCF & 25.84 & 18.64 & 12.53 & 52.96 & 37.13 &24.73\\
    ACRN & 24.22 &19.52 &14.62 &47.42 &34.97 &24.88\\
    ROLE & 20.37 &15.38& 9.94 &45.45 &31.17 &20.13\\
    VAL & 25.74 &19.76 &14.74 &51.87 &38.55 &26.52\\
    ACL-K & 31.64 &24.17 &20.01 &57.85 &42.15 &30.66\\
    CMIN & 32.48 &24.64 &18.05 &62.13 &38.46 &27.02\\
    QSPN & 25.31 &20.15 &15.23 &53.21 &36.72 &25.30\\
    SM-Rl & 26.51 &20.25 &15.95& 50.01 &38.47& 27.84\\
    SLTA & 23.13 &17.07 &11.92& 46.52 &32.90& 20.86\\
    ABLR & 34.70 &19.50 &9.40 & - & -&  -\\
    SAP & 31.15 & - &18.24 &53.51 & - &28.11\\
    TripNet & - &23.95 &19.17& -& - &-\\
    2D-TAN & \underline{47.59} &\underline{37.29} &\underline{25.32} &\underline{70.31} &\underline{57.81} &\underline{45.04}\\
    DRN & - & - & 23.17 & - & - & 33.36 \\
    DEBUG & - & 23.45 & 11.72 & - & - & -\\
    VSLNet & - & 29.61 & 24.27 & - & - & -\\
    \midrule
    Ours &  \textbf{53.59} & \textbf{43.09} & \textbf{32.24} & \textbf{79.83} & \textbf{68.71} & \textbf{55.51} \\ 
    \bottomrule
    \end{tabular}
    \caption{Performance comparison on TACoS. All results are reported in percentage (\%)}
    \label{tab:tacos}
\end{table}

\begin{table}[]
    \centering
    \begin{tabular}{ccccc}
    \toprule
    \multirow{2}{*}{\textbf{Methods}} &\multicolumn{2}{c}{\textbf{Rank1@}}& \multicolumn{2}{c}{\textbf{Rank5@}}\\
    & \textbf{0.5} & \textbf{0.7} & \textbf{0.5} & \textbf{0.7} \\
    \midrule
    \multicolumn{5}{c}{\textbf{VGG}}\\
    \midrule
    CTRL&23.63 &8.89&58.92 & 29.52 \\
    ACL-K& 30.48 &12.20 & 64.84& 35.13\\
    QSPN& 35.60 &15.80 & 79.40& 45.40 \\
    DEBUG & 37.39 & 17.69 & - &- \\
    MCN & 17.46 & 8.01 &48.22  & 26.73 \\
    ABLR& 24.36 &9.01 & -& -  \\
    SAP& 27.42 &13.36 & 66.37 & 38.15 \\
    MAN& 41.24 &20.54  & 83.21& 51.85 \\
    2D-TAN& 39.70 &23.31 & 80.32 & 51.26\\
    DRN&\underline{42.90} &\underline{23.68}  & \textbf{87.80} & \textbf{54.87} \\
    Ours& \textbf{44.33} & \textbf{26.59} & \underline{87.23}  & \underline{53.47} \\
    \midrule
    \multicolumn{5}{c}{\textbf{I3D}}\\
    \midrule
    ExCL& 44.10 & 22.40 & - &-\\
    VSLNet& \underline{54.19} & \underline{35.22} & -& -  \\
    DRN  & 53.09 & 31.50 & 89.06 & 60.05 \\
    Ours& \textbf{59.41} & \textbf{38.95} & \textbf{89.25} & \textbf{63.60}\\
    \bottomrule
    \end{tabular}
    \caption{Performance comparison on Charades-STA. All results are reported in percentage (\%)}
    \label{tab:sta}
\end{table}

\begin{table}[]
    \centering
    \begin{tabular}{ccccc}
    \toprule
    \multirow{2}{*}{\textbf{Methods}} & \multicolumn{2}{c}{\textbf{Rank1@}}  & \multicolumn{2}{c}{\textbf{Rank5@}} \\
    & \textbf{0.5} & \textbf{0.7} & \textbf{0.5} & \textbf{0.7} \\
    \midrule
    MCN & 21.36 & 6.43 & 53.23 & 29.70\\
    CTRL & 29.01 & 10.34 & 59.17 & 37.54 \\
    TGN & 27.93 & - & 44.20 & - \\
    ACRN & 31.67 & 11.25 & 60.34 & 38.57 \\
    CMIN & 44.62 & 24.48 & 69.66 & 52.96 \\
    QSPN & 33.26 & 13.43 & 62.39 & 40.78 \\
    ABLR & 36.79 & - & - & - \\
    TripNet & 32.19 & 13.93 & - & - \\
    PMI & 38.28 & 17.83 & - & - \\
    2D-TAN & 44.05 & \underline{27.38} & 76.65 & \underline{62.26} \\
    VSLNet & 43.22 & 26.16 & - & - \\
    DRN & \underline{45.45} & 24.39 & \textbf{77.97} & 50.30 \\
    ExCL & 42.7 & 24.1 & - & - \\
    DEBUG & 39.72 & - & - & - \\
    \midrule
    Ours & \textbf{46.23} & \textbf{29.37} & \underline{76.09} & \textbf{62.33} \\ 
    \bottomrule
    \end{tabular}
    \caption{Performance comparison on ActivityNet Captions. All results are reported in percentage (\%)}
    \label{tab:anet}
\end{table}

\subsubsection{Improvement on different IoUs}
In this section, we illustrate the performance gain achieved on ActivityNet Captions, TACoS and Charades-STA dataset in terms of different $\mu\in(0,1)$ with previous best method.

\begin{figure*}[t]
    \centering
    \includegraphics[width=1.0\linewidth]{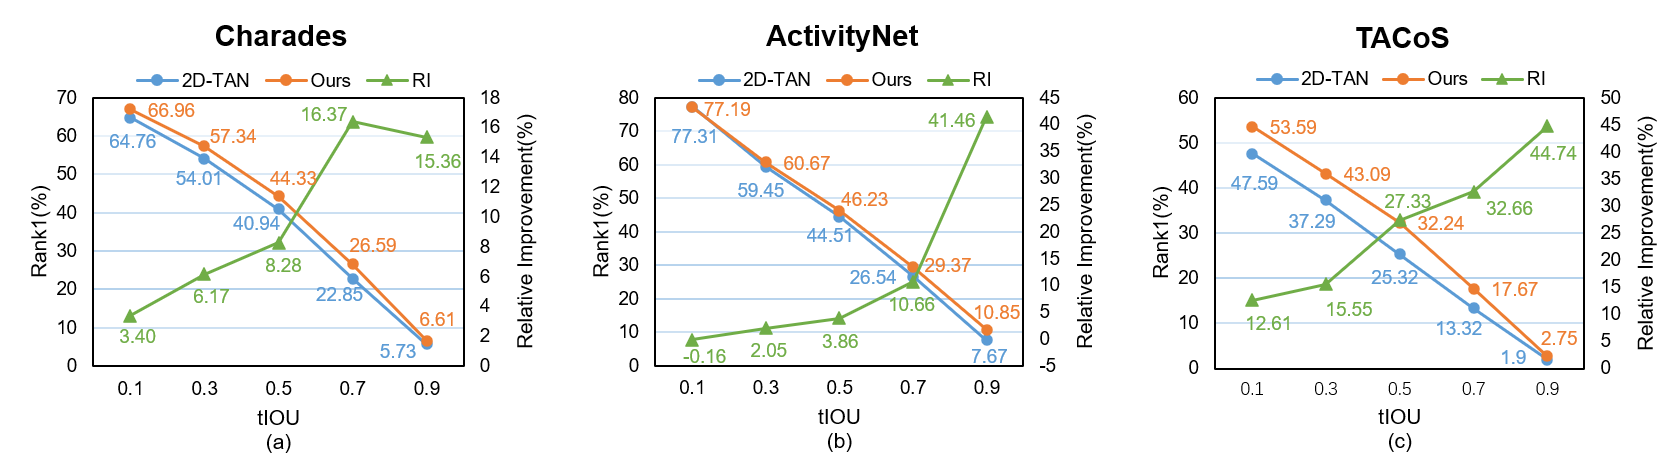}
    \caption{Detailed comparison across different IoU on three benchmarks in terms of \textit{Rank 1}}
    \label{fig:iou}
\end{figure*}
